# Supplementary material for: Towards Demystifying Representation Learning with Non-contrastive Self-supervision
Source: arXiv:2110.04947 source file (2022-09-26)
Supplement: Supplementary file 1 [file beyond_linear.tex]

\section{Beyond Linear Models: Limitations and Discussion}\label{sec:limitation}
\begin{figure}[h]
\centering
    \includegraphics[width=\linewidth]{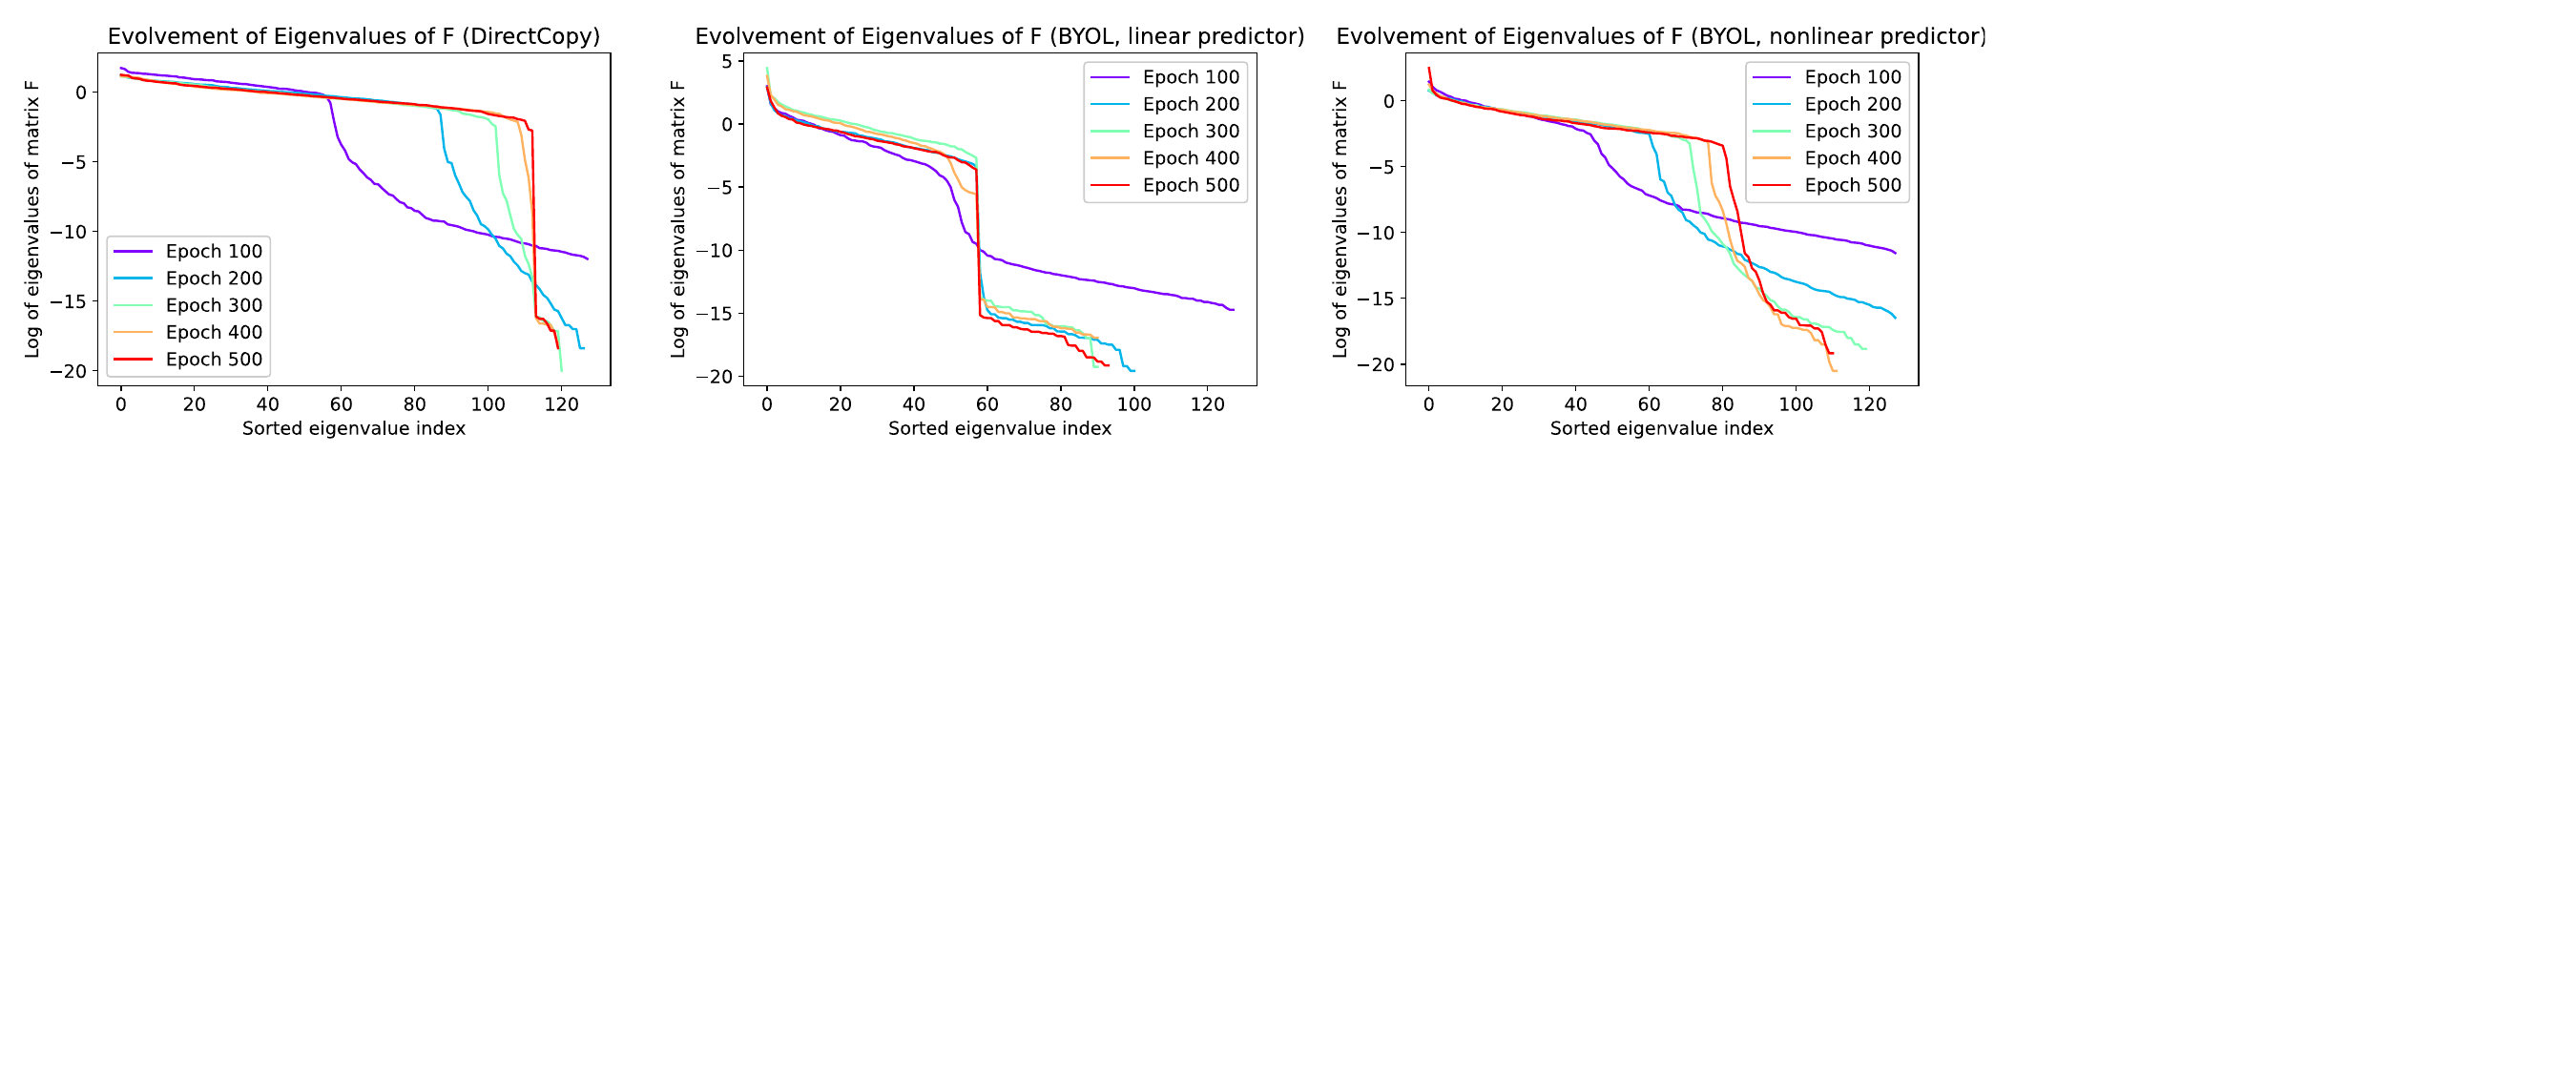}
\vspace{-0.5cm}
\caption{\small Eigenvalues of $F$ when trained by DirectCopy, BYOL with linear predictor and BYOL with two-layer nonlinear predictor on CIFAR-10 for different epochs. Top-1 accuracy at 500 epoch is 89.62 for DirectCopy, 88.83 for BYOL with linear predictor and 90.25 for BYOL with two-layer nonlinear predictor.}\label{fig:eigenvalues_eps_epoch}
\vspace{-0.3cm}
\end{figure}

\label{sec:discussion}
As a linear model used to study the behavior of \ncssl{}, our model does not capture all of its intriguing empirical phenomena. For example, we observed that the discarded nuisance features gradually come back after training over longer epochs. Moreover, whether it comes back or not is related to the downstream task performance. In Figure~\ref{fig:eigenvalues_eps_epoch} on CIFAR-10 dataset, both DirectCopy and BYOL with two-layer nonlinear predictor show this resurgence of nuisance features, as well as strong performance, while BYOL with linear predictor does not seem to learn new features even when trained longer, which might explain its worse performance. %We also observed similar phenomenon on STL-10 with even a larger gap in performance: DirectCopy achieves 82.95 top-1 accuracy at epoch 500, BYOL with linear predictor gets 78.23 and BYOL with two-layer nonlinear predictor gets 84.00.

One conjecture is that at the beginning of training, weight decay prioritize the invariant features (i.e., low variance under augmentation) over nuisance ones. The invariant features then grow, building their own supporting low-level features. After that, the nuisance feature, which is also useful, are gradually picked up in later stage. Since the low-level features are already trained through previous steps of back-propagation, the nuisance features are encouraged to use them as the supporting features, rather than creating their own. In contrast, if we train both the invariant and nuisance features simultaneously, they will \emph{compete} over the limited pool of low-level supporting features defined by the capacity of the network, leading to worse learned representations. We believe understanding these phenomena require analysis on the non-linear networks, and we leave it as future work.
